# Supplementary material for: You Are What You Talk About: Inducing Evaluative Topics for Personality Analysis
Source: arXiv:2302.00493 source file (2023-02-01)
Supplement: Supplementary file 1 [file cluster_table.tex]

\begin{table*}
\centering
\small
\begin{tabular}{ll}
\toprule
Evaluative topic & Representants \\
\midrule 
open & people, lot, free, good, permit, time, going, open, big, trying \\
food/drinks & taste, meat, smell, beer, texture, flavour, savory, drink, palate, sweet \\
religion & testimony, believe, truth, god, witness, primordial, bible, church, jesus, earth \\
demeaning & shit, tell, talking, strangers, rude, stupid, bitch, upset, weird, shitty \\
investing/finance & recommend, pack, vouch, opt, buying, invest, fund, ticket, stock, dealt \\
fiction & watch, character, read, movies, story, books, thought, cool, new, anime \\
music & songs, album, pop, favourite, music, voice, listen, lyrics, track, sound \\
gaming & play, game, level, team, damage, skill, hit, gear, combat, dungeons \\
social issues & society, human, religion, culture, rights, moral, white, argument, victimhood, black \\
hatred & despise, hate, passion, stand, fucking, goddamn, nerd, mad, smug, ads \\
day-to-day & day, work, hours, week, spend, food, money, sleep, home, eat \\
relationships & relationship, woman, dating, child, partner, man, sex, ex, gay, alimony \\
argument & opinion, salt, grain, sanctimonious, worthless, controversial, assessment, disclaimer, 180, nuanced \\
political & government, party, vote, trump, support, country, state, speaker, system, tax \\
sexual/looks & hot, hair, sexy, gross, facial, body, attractive, wear, porn, dimorphism \\
personality & type, personality, mbti, emotions, test, cognitive, learning, ideas, brain, jung \\
debate & understand, discussion, post, saying, person, wrong, think, point, internet, debate \\
maltreatment & despised, hated, school, dropped, sucked, harass, refuses, skipped, hood, beaten \\
occult & fate, chime, cat, spirits, guides, luck, desperately, talisman, invite, mirror \\
\bottomrule
\end{tabular}
\caption{Evaluative topics produced by CTM. The last column lists facets that correlate to the corresponding evalutive topic with statistical significance ($p < .01)$. Facets in bold signify positive correlations, and those in italic denote negative correlations. We incorporated correction for the false discovery rate, namely the Benjamini-Hochberg method, due to multiple correlation tests. We calculated the p-values based on the Fisher's z-transformation of correlations.}
\label{tab:cluster_full}
\end{table*}
