# Supplementary material for: You Are What You Talk About: Inducing Evaluative Topics for Personality Analysis
Source: arXiv:2302.00493 source file (2023-02-01)
Supplement: Supplementary file 2 [file qsb_algo.tex]

% algorithm2e settings
\DontPrintSemicolon
\LinesNumbered
\SetAlgoLined

% PSEUDOCODE START
\begin{algorithm}
\caption{Quasi-Snowballing}
\label{alg:qsb}
\KwData{sentence embeddings $\mathcal{D}$; seed set embeddings $\mathcal{S}$; similarity threshold $t_{sim}$; temperature factor $\gamma$}
\KwResult{snowballed set $\mathcal{P}$}
\SetKwRepeat{Do}{do}{while}
$\mathcal{P} \leftarrow \emptyset$ \;
$\mathcal{P} \leftarrow \mathcal{P} \cup \mathcal{S}$ \;
\Do{$\mathcal{H} \neq \emptyset$}{
    $\mathcal{C} \leftarrow \mathcal{D} \setminus \mathcal{P}$ \tcp*[f]{candidate set} \;
    $\mathcal{H}$ = \textit{cosineSimilarityHits}($\mathcal{C}, \mathcal{P}, t_{sim}$) \;
    $\mathcal{P} \leftarrow \mathcal{P} \cup \mathcal{H} $ \;
    $t_{sim} \leftarrow \gamma t_{sim}$ \tcp*[f]{annealing} \;
}
\Return $\mathcal{P}$
\end{algorithm}
% PSEUDOCODE END
